# Supplementary material for: Pseudo-Goldstone modes and dynamical gap generation from order-by-thermal-disorder
Source: arXiv:2301.11948 source file (2023-07-06)
Supplement: Supplementary file 1 [file supp.pdf]

# Supplemental Material for "Pseudo-Goldstone modes and dynamical gap generation from order-by-thermal-disorder"


Subhankar Khatua,[1,2] Michel J. P. Gingras,[2] and Jeffrey G. Rau[1]

[1]*Department of Physics, University of Windsor, 401 Sunset Avenue, Windsor, Ontario, N9B 3P4, Canada*
[2]*Department of Physics and Astronomy, University of Waterloo, Waterloo, Ontario, N2L 3G1, Canada*



(Dated: July 6, 2023)


## I. DETAILS OF MONTE CARLO SIMULATIONS

### A. Details of Monte Carlo procedure

The Monte Carlo (MC) simulations described in the main text are based on adaptive single-site Metropolis moves [1], combined with over-relaxation moves [2]. A typical single-site Metropolis move involves randomly selecting a spin and changing its orientation to a random direction. However, at low temperature, most such moves result in configurations that are of much higher energies and thus rejected [3]. Therefore, we follow an adaptive approach that selects a spin randomly and changes its orientation to a Gaussian distributed random direction *within a solid-angle of certain width*. The solid-angle-width changes adaptively to ensure that the update-acceptance rate remains close to 50% at each temperature (see Ref. [1] for details). The over-relaxation move rotates a randomly selected spin by a random angle about its local exchange field. This move is energy-conserving and thus always accepted. We define a Monte Carlo sweep at a certain temperature as a combination of $N$ (total number of spins) random successive adaptive single-site Metropolis moves with each followed by five random over-relaxation moves. All the simulation results discussed in the main text have been obtained by considering periodic boundary conditions on a square lattice of size $L$ by $L$ and $N = L^2$ spins. As in the main text, we use units such that $J = \hbar = k_{\rm B} = 1$.

### B. Simulation details of the order parameter distribution

Starting from a random spin configuration at high temperature, $T = 10$ (larger than $K$) where the system is in the paramagnetic phase, we slowly cool down in steps of size $\delta T = 0.1$ to a final temperature $T = 0.4$ (much smaller than $K$). At each temperature, we perform $10^5$ MC sweeps to equilibrate the system. Finally, at $T = 0.4$, after thermal equilibration has been achieved, we record the net magnetization-per-spin over $10^6$ MC samples, leaving five MC sweeps in between two consecutive measurements. From the net magnetization per spin, $\boldsymbol{M} = (M_x, M_y, M_z)$, we calculate $\phi = \arctan(M_y/M_x)$, computing a distribution for $\phi$. Since the ferromagnetic Heisenberg-compass model has a global $C_4$ rotation symmetry in the $\hat{\boldsymbol{x}} - \hat{\boldsymbol{y}}$ plane, we symmetrize the distribution by shifting the data by $\pi/2$, $\pi$, and $3\pi/2$ , i.e., add $\pi/2$, $\pi$, and $3\pi/2$ to each entry of the dataset. We have plotted the final dataset as a probability density, $P(\phi)$ for $\phi \in [-\pi/4, \pi/4]$ with 50 bins for three different system sizes, $N = 6^2, 10^2$, and $14^2$ in Fig. 1(a) in the main text. We have chosen a large value for $K$, i.e., $K = 5$, for all simulations in order to achieve a strong thermal order-by-disorder selection effect at accessible system sizes. For the gross spectral features, the largest system size considered for spin-dynamics simulations was $N = 100^2$, while for detailed features, such as the temperature dependence of the pseudo-Goldstone (PG) gap, up to $N = 40^2$ was used. Had smaller values of $K$ been used, all the MC simulations, as well as spin-dynamics simulations, would have had to be performed for much larger system sizes to obtain results that converge when system size is extrapolated to the thermodynamic limit ($N \to \infty$).

### C. Simulation details of magnetization and its derivative with respect to temperature

Independently at each temperature $T$, $5 \times 10^5$ MC sweeps are performed on a perfectly aligned ferromagnetic spin configuration along $\hat{\boldsymbol{x}}$ for equilibration, followed by $3 \times 10^6$ successive MC sweeps to measure the net magnetization per spin along $\hat{\boldsymbol{x}}$ ($M$), total energy ($E$), and their product ($EM$). Their product is recorded in order to calculate the derivative of the magnetization(-per-spin) with respect to temperature, given by

$$\frac{\partial M}{\partial T} \equiv \frac{\langle EM\rangle - \langle E\rangle\langle M\rangle}{T^2}, \tag{S1}$$

where $\langle x\rangle$ is the MC thermal average of quantity $x$. To estimate the statistical errors on static quantities, the $3 \times 10^6$ measurements are divided into 30 blocks, and then resampled using the standard bootstrap method [3]. Typically, $O(10^3)$ bootstrap samples were generated from these blocks to estimate the statistical errors. In Fig. 3 of the main text, the error bars shown correspond to twice the standard deviation estimated via bootstrap.

## II. DETAILS OF SPIN-DYNAMICS SIMULATIONS

Numerical integrations of the Landau-Lifshitz equations have been done using an adaptive step size RK5(4) Dormand-Prince integrator [4] from the Boost-Odeint C++ library [5, 6]. The initial spin configurations for the numerical integration are generated from MC simulations described in Sec. I.

To obtain the results shown in Fig. 1(b) in the main text, we perform $5 \times 10^5$ equilibration MC sweeps on a perfectly aligned ferromagnetic configuration along $\hat{\boldsymbol{x}}$ at $T = 0.4$. Starting from the final state, we perform another $15 \times 10^3$ MC

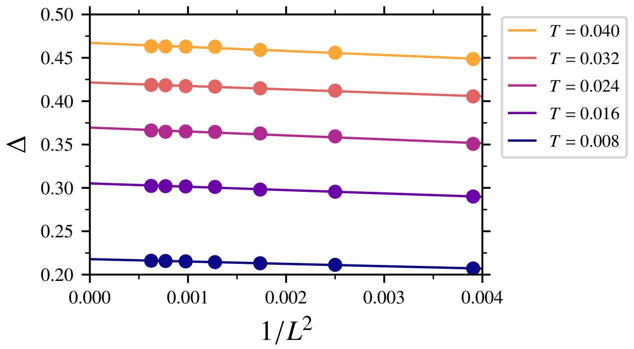


FIG. S1. Finite size scaling of the PG gap obtained from spin-dynamics simulations for several temperatures ($K = 5$).

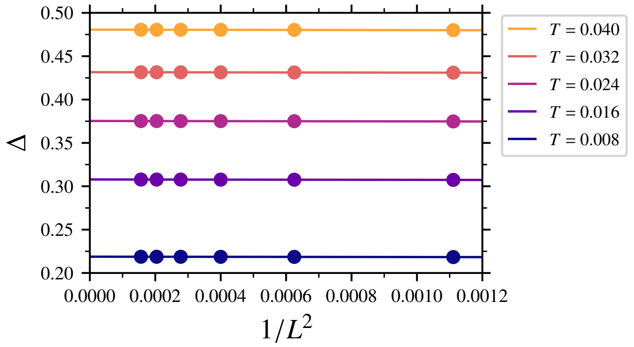


FIG. S2. Finite size scaling of the PG gap obtained using SCMFT for several temperatures ($K = 5$).

sweeps for 350 independent parallel runs to generate well-equilibrated configurations at $T = 0.4$. Next, we feed each of these 350 configurations into the Dormand-Prince integrator as an initial state and integrate to a final time, $t_{\max} = 50$. The error tolerance of the integrator is set to $10^{-8}$, such that the energy-per-spin and individual spin lengths are conserved to at least one part in $10^7$ and $10^{10}$, respectively. For each of these independent 350 integrations, we calculate the Fourier

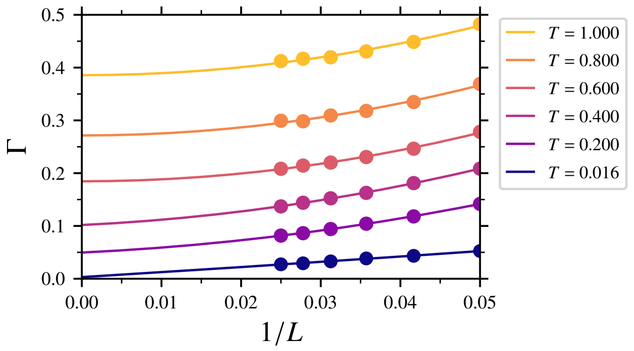


FIG. S3. Finite size scaling of the PG linewidth obtained from spin-dynamics simulations for several temperatures ($K = 5$).

transform of the spin configurations in space and time, $\boldsymbol{S}(\boldsymbol{k}, \omega)$ using the C++ FFTW++ [7] library and then compute the dynamical structure factor, $\mathcal{S}(\boldsymbol{k}, \omega) = |\boldsymbol{S}(\boldsymbol{k}, \omega)|^2$, finally taking an average of the structure factors found from the 350 initial configurations to obtain Fig. 1(b).

The results in Fig. 1(c) in the main text are obtained as follows: The system is initialized in a perfectly aligned ferromagnetic configuration along $\hat{\boldsymbol{x}}$ at a temperature $T = 0.0004$, and slowly warmed up in steps of $\delta T = 0.0004$ to a temperature $T = 0.04$. At each temperature, we perform $10^5$ equilibration MC sweeps, generating a configuration at $T = 0.008, 0.016, 0.024, 0.032, 0.04$. At each of these temperatures, we then apply the following procedure. Starting from a given spin configuration, say at $T = 0.008$, we generate a total of $2 \times 10^3$ configurations independently by performing $10^5$ MC sweeps. Each of these configurations is fed into the Dormand-Prince integrator independently to integrate to a final time, $t_{\max} = 2500$. Note that this $t_{\max}$ value is taken to be much larger than the $t_{\max} = 50$ value used to obtain the results shown in Fig. 1(b). As discussed in the main text, to determine the PG gap, $\Delta$, and linewidth, $\Gamma$, a much higher frequency resolution is needed and thus the total integration time must be significantly larger. The error tolerance of the integrator is set to $10^{-10}$, such that the energy-per-spin and spin-length are conserved to at least one part in $10^8$ and $10^{10}$, respectively. After the time evolution, we compute the Fourier transform of the spin configurations in space and time using FFTW++ and then compute the dynamical structure factor, $\mathcal{S}(\boldsymbol{k}, \omega)$. Finally, we perform an average over the $2 \times 10^3$ initial spin configurations to obtain the average dynamical structure factor at $T = 0.008$. In Fig. 1(c), we show only a cut of the average dynamical structure factor at the zone center, $\mathcal{S}(\mathbf{0}, \omega)$. To clearly visualize $\mathcal{S}(\mathbf{0}, \omega)$ at several different temperatures in a single plot, we stagger them on the $y$-axis by a fixed offset between the $\mathcal{S}(\mathbf{0}, \omega)$ data at two consecutive temperatures.

To obtain the results shown in Fig. 2 of the main text, we proceed as follows: At each temperature, we follow the same method as described for Fig. 1(c) in the previous paragraph and compute $\mathcal{S}(\mathbf{0}, \omega)$ for several system sizes, $L = 20, 24, 28, 32, 36$, and 40. To find the gap and linewidth for each system size, we fit each data to a Gaussian (a Gaussian lineshape fits the data in the range $T \leq 0.04$ best, compared to, e.g., a Lorentzian). The center of the Gaussian is used to define the PG gap and the full-width at half maximum (FWHM) of the Gaussian, i.e., $2.355\sigma$ ($\sigma$ being the standard deviation), is taken as the PG linewidth. Finite size $L$-dependent PG gaps and linewidths are then extrapolated in system size ($L \to \infty$) to obtain the corresponding values in the thermodynamic limit. Finite size scaling behavior of the PG gap is shown in Fig. S1. The finite size scaling of the PG gap obtained using the self-consistent mean-field theory (SCMFT) is shown in Fig. S2 (See Sec. III E below for details).

At very low temperatures, e.g., $T \leq 0.04$, where $\mathcal{S}(\mathbf{0}, \omega)$ falls very sharply away from the center of the peak, a Gaussian lineshape is a natural choice. However, as temperature increases further, $\mathcal{S}(\mathbf{0}, \omega)$ shows more pronounced tails and a Lorentzian lineshape was found to provide a better description of the data. Finite size scaling of the PG linewidth is

shown in Fig. S3. At $T = 0.016$, the PG linewidths for different system sizes are found by fitting to a Gaussian while for the remaining temperatures in Fig. S3, the PG linewidths are found from fitting to Lorentzian (via the FWHM of the corresponding Lorentzian). Finite size scaling reveals that at very low temperatures, the PG linewidth scales almost linearly with $1/L$ with the scaling becoming quadratic in $1/L$ as temperature increases (see Fig. S3).

## III. SPIN WAVE THEORY

Here, we elaborate on the formalism for interacting spin waves in the ferromagnetic Heisenberg-compass model on the square lattice. We consider the Heisenberg-compass model Hamiltonian

$$\mathcal{H} = -\sum_{\boldsymbol{r},\delta}\left[J\boldsymbol{S}_{\boldsymbol{r}}\cdot\boldsymbol{S}_{\boldsymbol{r}+\boldsymbol{\delta}} + KS^{\delta}_{\boldsymbol{r}}S^{\delta}_{\boldsymbol{r}+\boldsymbol{\delta}}\right] \equiv \sum_{\boldsymbol{r},\delta}\boldsymbol{S}^{\intercal}_{\boldsymbol{r}}\boldsymbol{J}_{\delta}\boldsymbol{S}_{\boldsymbol{r}+\boldsymbol{\delta}}, \tag{S2}$$

where $\boldsymbol{\delta} = \boldsymbol{x}, \boldsymbol{y}$ denotes the nearest-neighbour (horizontal and vertical) bonds. For $J > 0$ and $K > 0$, the classical ground state is ferromagnetic and has an accidental degeneracy parametrized by an angle $\phi$

$$\boldsymbol{S}_{\boldsymbol{r}} = S(\cos\phi\,\hat{\boldsymbol{x}} + \sin\phi\,\hat{\boldsymbol{y}}). \tag{S3}$$

For small $|K|$ and $K < 0$, one finds only a (symmetry-enforced) discrete degeneracy, with $\boldsymbol{S}_{\boldsymbol{r}} = \pm S\,\hat{\boldsymbol{z}}$. For large $|K|$ and $K < 0$, the ground state is described by an $XY$-stripe phase parametrized by a single angle whose two extreme limits are an $X$-stripe phase (i.e., all spins are lying along the $\hat{\boldsymbol{x}}$ axis, arranging themselves antiferromagnetically along the $\hat{\boldsymbol{x}}$ axis and ferromagnetically along the $\hat{\boldsymbol{y}}$ axis) and a $Y$-stripe phase (i.e., all spins are lying along the $\hat{\boldsymbol{y}}$ axis, arranging themselves antiferromagnetically along the $\hat{\boldsymbol{y}}$ axis and ferromagnetically along the $\hat{\boldsymbol{x}}$ axis). The phases for $J < 0$ can be obtained by mapping $\boldsymbol{S}_{\boldsymbol{r}} \to (-1)^{\boldsymbol{r}}\boldsymbol{S}_{\boldsymbol{r}}$ which alternates on the two sublattices. We note that the dynamics however differ between $J > 0$ and $J < 0$, since the sign change on one sublattice is not a canonical transformation.

Returning to the $J > 0$, $K > 0$ case, we define a frame aligned with a ferromagnetic ground state whose magnetization direction is parametrized with an angle $\phi$

$$\hat{\boldsymbol{e}}_x = -\sin\phi\,\hat{\boldsymbol{x}} + \cos\phi\,\hat{\boldsymbol{y}}, \quad \hat{\boldsymbol{e}}_y = \hat{\boldsymbol{z}}, \quad \hat{\boldsymbol{e}}_z = \cos\phi\,\hat{\boldsymbol{x}} + \sin\phi\,\hat{\boldsymbol{y}},$$

as well as $\hat{\boldsymbol{e}}_{\pm} \equiv (\hat{\boldsymbol{e}}_x \pm i\hat{\boldsymbol{e}}_y)/\sqrt{2}$ and $\hat{\boldsymbol{e}}_0 \equiv \hat{\boldsymbol{e}}_z$. Here, $\hat{\boldsymbol{x}}$, $\hat{\boldsymbol{y}}$ and $\hat{\boldsymbol{z}}$ are the global Cartesian axes. We then have the *local exchanges* $\mathcal{J}^{\mu\nu}_{\delta} = \hat{\boldsymbol{e}}^{\intercal}_{\mu}\boldsymbol{J}_{\delta}\hat{\boldsymbol{e}}_{\nu}$. The Fourier transforms of the exchange matrix elements, $\mathcal{J}^{\mu\nu}_{\delta}$, are defined as $\mathcal{J}_{\boldsymbol{k}} \equiv \sum_{\delta} 2\cos(\boldsymbol{k}\cdot\boldsymbol{\delta})\mathcal{J}_{\delta}$ where the fact that $-\boldsymbol{\delta}$ and $\boldsymbol{\delta}$ are equivalent has been used. Explicitly, these are given by

$$\begin{aligned}
\mathcal{J}^{+-}_{\boldsymbol{k}} &= -\left(2J + K\sin^2\phi\right)\cos k_x - \left(2J + K\cos^2\phi\right)\cos k_y,\\
\mathcal{J}^{00}_{\boldsymbol{k}} &= -2\left(J + K\cos^2\phi\right)\cos k_x - 2\left(J + K\sin^2\phi\right)\cos k_y,\\
\mathcal{J}^{++}_{\boldsymbol{k}} &= -\left(K\sin^2\phi\right)\cos k_x - \left(K\cos^2\phi\right)\cos k_y,\\
\mathcal{J}^{0\pm}_{\boldsymbol{k}} &= -\frac{K}{\sqrt{2}}\sin(2\phi)\left(\cos k_y - \cos k_x\right),
\end{aligned}$$

with $\mathcal{J}^{-+}_{\boldsymbol{k}} = [\mathcal{J}^{+-}_{\boldsymbol{k}}]^*$, $\mathcal{J}^{--}_{\boldsymbol{k}} = [\mathcal{J}^{++}_{\boldsymbol{k}}]^*$ and $\mathcal{J}^{0\pm}_{\boldsymbol{k}} = \mathcal{J}^{\pm 0}_{\boldsymbol{k}}$. Note that $\mathcal{J}^{00}_{0} = -2(2J + K)$. For one of the four ground states selected by order-by-thermal-disorder (ObTD), e.g. $\phi = 0$, these $\mathcal{J}^{\mu\nu}_{\boldsymbol{k}}$ are given by

$$\begin{aligned}
\mathcal{J}^{+-}_{\boldsymbol{k}} &= -2J\cos k_x - (2J + K)\cos k_y,\\
\mathcal{J}^{00}_{\boldsymbol{k}} &= -2(J + K)\cos k_x - 2J\cos k_y,\\
\mathcal{J}^{++}_{\boldsymbol{k}} &= -K\cos k_y,\\
\mathcal{J}^{0\pm}_{\boldsymbol{k}} &= 0.
\end{aligned}$$

Performing the usual Holstein-Primakoff expansion [8] to $O(S^0)$ on this model yields [9]

$$\mathcal{H} \approx E_0 + \mathcal{H}_2 + (\mathcal{H}_{4,2-2} + \mathcal{H}_{4,3-1} + \mathcal{H}_{4,1-3}) + \cdots, \tag{S4}$$

where we have defined the constant classical part $E_0 = -NS^2(2J + K)$ [at $O(S^2)$] and

$$\mathcal{H}_2 = \sum_{\boldsymbol{k}}\left[A_{\boldsymbol{k}}a^{\dagger}_{\boldsymbol{k}}a_{\boldsymbol{k}} + \frac{1}{2!}\left(B_{\boldsymbol{k}}a^{\dagger}_{\boldsymbol{k}}a^{\dagger}_{-\boldsymbol{k}} + B^*_{\boldsymbol{k}}a_{-\boldsymbol{k}}a_{\boldsymbol{k}}\right)\right], \tag{S5a}$$

$$\mathcal{H}_{4,2-2} = \frac{1}{N}\sum_{\boldsymbol{k}\boldsymbol{k}'\boldsymbol{q}}\frac{1}{(2!)^2}V_{\boldsymbol{k},\boldsymbol{k}',\boldsymbol{q}}a^{\dagger}_{\boldsymbol{k}+\boldsymbol{q}}a^{\dagger}_{\boldsymbol{k}'-\boldsymbol{q}}a_{\boldsymbol{k}'}a_{\boldsymbol{k}}, \tag{S5b}$$

$$\mathcal{H}_{4,3-1} = \frac{1}{N}\sum_{\boldsymbol{k}\boldsymbol{k}'\boldsymbol{q}}\frac{1}{3!}D_{\boldsymbol{k},\boldsymbol{k}',\boldsymbol{q}}a^{\dagger}_{\boldsymbol{k}}a^{\dagger}_{\boldsymbol{k}'}a^{\dagger}_{\boldsymbol{q}}a_{\boldsymbol{k}+\boldsymbol{k}'+\boldsymbol{q}} = \mathcal{H}^{\dagger}_{4,1-3}. \tag{S5c}$$

This includes the quadratic parts [at $O(S)$] in $\mathcal{H}_2$ as well as the quartic parts [at $O(S^0)$] in $\mathcal{H}_4 \equiv \mathcal{H}_{4,2-2} + \mathcal{H}_{4,3-1} + \mathcal{H}_{4,1-3}$. The quartic part has been decomposed into a $2-2$ scattering term, $\mathcal{H}_{4,2-2}$, and anomalous $3-1$ and $1-3$ terms, $\mathcal{H}_{4,3-1}$ and $\mathcal{H}_{4,1-3}$. Since $\mathcal{J}^{0,\pm}_{\boldsymbol{k}} = 0$, there are no three boson terms in $\mathcal{H}$ [Eq. (S4)]. In terms of the local exchanges, the coefficients in $\mathcal{H}_2$ and $\mathcal{H}_4$ are given explicitly by

$$\begin{aligned}
A_{\boldsymbol{k}} &= S\left(\mathcal{J}^{+-}_{\boldsymbol{k}} - \mathcal{J}^{00}_{\boldsymbol{0}}\right),\\
B_{\boldsymbol{k}} &= S\mathcal{J}^{++}_{\boldsymbol{k}},\\
V_{\boldsymbol{k},\boldsymbol{k}',\boldsymbol{q}} &= \frac{1}{2}\left(\mathcal{J}^{00}_{\boldsymbol{k}'-\boldsymbol{k}-\boldsymbol{q}} + \mathcal{J}^{00}_{-\boldsymbol{q}} + \mathcal{J}^{00}_{+\boldsymbol{q}} + \mathcal{J}^{00}_{\boldsymbol{k}-\boldsymbol{k}'+\boldsymbol{q}}\right)\\
&\quad - \frac{1}{2}\left(\mathcal{J}^{+-}_{\boldsymbol{k}} + \mathcal{J}^{+-}_{\boldsymbol{k}'} + \mathcal{J}^{+-}_{\boldsymbol{k}'-\boldsymbol{q}} + \mathcal{J}^{+-}_{\boldsymbol{k}+\boldsymbol{q}}\right),\\
D_{\boldsymbol{k},\boldsymbol{k}',\boldsymbol{q}} &= -\frac{1}{2}\left(\mathcal{J}^{++}_{\boldsymbol{k}} + \mathcal{J}^{++}_{\boldsymbol{k}'} + \mathcal{J}^{++}_{\boldsymbol{q}}\right).
\end{aligned}$$

By construction, these coefficients must satisfy the following symmetry relations

$$\begin{aligned}
A_{\boldsymbol{k}} &= A^*_{\boldsymbol{k}},\\
B_{\boldsymbol{k}} &= B_{-\boldsymbol{k}},\\
V_{\boldsymbol{k},\boldsymbol{k}',\boldsymbol{q}} &= V_{\boldsymbol{k}',\boldsymbol{k},-\boldsymbol{q}} = V_{\boldsymbol{k},\boldsymbol{k}',\boldsymbol{k}'-\boldsymbol{k}-\boldsymbol{q}} = V_{\boldsymbol{k}',\boldsymbol{k},\boldsymbol{k}-\boldsymbol{k}'+\boldsymbol{q}} = V^*_{\boldsymbol{k}+\boldsymbol{q},\boldsymbol{k}'-\boldsymbol{q},-\boldsymbol{q}},\\
D_{\boldsymbol{k},\boldsymbol{k}',\boldsymbol{q}} &= D_{\boldsymbol{k},\boldsymbol{q},\boldsymbol{k}'} = D_{\boldsymbol{k}',\boldsymbol{k},\boldsymbol{q}} = D_{\boldsymbol{k}',\boldsymbol{q},\boldsymbol{k}} = D_{\boldsymbol{q},\boldsymbol{k},\boldsymbol{k}'} = D_{\boldsymbol{q},\boldsymbol{k}',\boldsymbol{k}}.
\end{aligned}$$

### A. Non-interacting spin-waves

We first consider only the quadratic (non-interacting magnon) portion of $\mathcal{H}$,

$$\mathcal{H}_2 = \sum_{\boldsymbol{k}}\left[A_{\boldsymbol{k}}a^{\dagger}_{\boldsymbol{k}}a_{\boldsymbol{k}} + \frac{1}{2!}\left(B_{\boldsymbol{k}}a^{\dagger}_{\boldsymbol{k}}a^{\dagger}_{-\boldsymbol{k}} + \text{H.c.}\right)\right]. \tag{S6}$$

This can be diagonalized by the usual Bogoliubov transformation [8]. Defining the matrix

$$\boldsymbol{M}_{\boldsymbol{k}} \equiv \begin{pmatrix} A_{\boldsymbol{k}} & B_{\boldsymbol{k}} \\ B^*_{\boldsymbol{k}} & A_{\boldsymbol{k}} \end{pmatrix}, \tag{S7}$$

the spin-wave spectrum is obtained by diagonalization of $\boldsymbol{\sigma}_z \boldsymbol{M}_{\boldsymbol{k}}$, where $\boldsymbol{\sigma}_z$ is a (block) Pauli matrix. One finds the positive frequency mode

$$\omega_{\boldsymbol{k}} = \sqrt{A^2_{\boldsymbol{k}} - |B_{\boldsymbol{k}}|^2} > 0.$$

For the ferromagnetic Heisenberg-compass model, $A_{\boldsymbol{k}}$ and $B_{\boldsymbol{k}}$ are given by

$$A_{\boldsymbol{k}} = -S\left[\left(2J + K\sin^2\phi\right)\cos k_x + \left(2J + K\cos^2\phi\right)\cos k_y - 2(2J+K)\right]$$

$$B_{\boldsymbol{k}} = -S\left[\left(K\sin^2\phi\right)\cos k_x + \left(K\cos^2\phi\right)\cos k_y\right].$$

Note that $A_{\boldsymbol{0}} = KS$ and $B_{\boldsymbol{0}} = -KS$, yielding a zero energy mode at $\boldsymbol{k} = \boldsymbol{0}$, with $\omega_{\boldsymbol{0}} = 0$ and with both $A_{\boldsymbol{k}}$ and $B_{\boldsymbol{k}}$ real. The eigenvector of $\boldsymbol{\sigma}_z \boldsymbol{M}_{\boldsymbol{k}}$ associated with the positive mode can be written as $(u_{\boldsymbol{k}}, v_{\boldsymbol{k}})$ where

$$u_{\boldsymbol{k}} = \sqrt{\frac{\omega_{\boldsymbol{k}} + A_{\boldsymbol{k}}}{2\omega_{\boldsymbol{k}}}}, \qquad v_{\boldsymbol{k}} = -\frac{B_{\boldsymbol{k}}}{\sqrt{2\omega_{\boldsymbol{k}}(\omega_{\boldsymbol{k}} + A_{\boldsymbol{k}})}},$$

which we have defined so that $u^2_{\boldsymbol{k}} - v^2_{\boldsymbol{k}} = 1$. Note that since both $A_{\boldsymbol{k}}$ and $B_{\boldsymbol{k}}$ are inversion even, we have $u_{-\boldsymbol{k}} = u_{\boldsymbol{k}}$, $v_{-\boldsymbol{k}} = v_{\boldsymbol{k}}$ and $\omega_{\boldsymbol{k}} = \omega_{-\boldsymbol{k}}$. Since both $A_{\boldsymbol{k}}$ and $B_{\boldsymbol{k}}$ are real, we find that $u_{\boldsymbol{k}}$ and $v_{\boldsymbol{k}}$ are real as well. The diagonalized boson operators are defined via

$$a_{\boldsymbol{k}} = u_{\boldsymbol{k}}\gamma_{\boldsymbol{k}} + v_{\boldsymbol{k}}\gamma^\dagger_{-\boldsymbol{k}}, \qquad a^\dagger_{\boldsymbol{k}} = v_{\boldsymbol{k}}\gamma_{-\boldsymbol{k}} + u_{\boldsymbol{k}}\gamma^\dagger_{\boldsymbol{k}}.$$

Expectation values of bilinears of these bosons can be written in terms of $u_{\boldsymbol{k}}$ and $v_{\boldsymbol{k}}$. Noting that at temperature $T$ these are

$$\langle\gamma^\dagger_{\boldsymbol{k}}\gamma_{\boldsymbol{k}}\rangle = n_{\rm B}(\omega_{\boldsymbol{k}}), \qquad \langle\gamma_{\boldsymbol{k}}\gamma^\dagger_{\boldsymbol{k}}\rangle = 1 + n_{\rm B}(\omega_{\boldsymbol{k}}),$$

where $n_{\rm B}(\omega) = [\exp(\omega/T) - 1]^{-1}$ is the boson thermal occupation number. The above thermal expectations for the original $a$-bosons are given by

$$\langle a^\dagger_{\boldsymbol{k}} a_{\boldsymbol{k}}\rangle = n_{\rm B}(\omega_{\boldsymbol{k}}) u^2_{\boldsymbol{k}} + [1 + n_{\rm B}(\omega_{\boldsymbol{k}})]\, v^2_{\boldsymbol{k}},$$

$$\langle a_{\boldsymbol{k}} a_{-\boldsymbol{k}}\rangle = \langle a^\dagger_{-\boldsymbol{k}} a^\dagger_{\boldsymbol{k}}\rangle^* = [1 + 2n_{\rm B}(\omega_{\boldsymbol{k}})]\, u_{\boldsymbol{k}} v_{\boldsymbol{k}}.$$

In the classical limit, where $T \gg \omega_{\boldsymbol{k}}$, we have $n_{\rm B}(\omega_{\boldsymbol{k}}) \approx T/\omega_{\boldsymbol{k}} \gg 1$. The expectations then become

$$\langle a^\dagger_{\boldsymbol{k}} a_{\boldsymbol{k}}\rangle = \frac{T}{\omega_{\boldsymbol{k}}}\left(u^2_{\boldsymbol{k}} + v^2_{\boldsymbol{k}}\right) = \frac{T}{\omega_{\boldsymbol{k}}}\left(\frac{A_{\boldsymbol{k}}}{\omega_{\boldsymbol{k}}}\right), \tag{S8a}$$

$$\langle a_{\boldsymbol{k}} a_{-\boldsymbol{k}}\rangle = \langle a^\dagger_{-\boldsymbol{k}} a^\dagger_{\boldsymbol{k}}\rangle = \frac{2T}{\omega_{\boldsymbol{k}}} u_{\boldsymbol{k}} v_{\boldsymbol{k}} = -\frac{T}{\omega_{\boldsymbol{k}}}\left(\frac{B_{\boldsymbol{k}}}{\omega_{\boldsymbol{k}}}\right). \tag{S8b}$$

Finally, the ordered moment (selected by ObTD), $\boldsymbol{M} \equiv \frac{1}{N}\sum_{\boldsymbol{r}}\langle \boldsymbol{S}_{\boldsymbol{r}}\rangle \equiv M\hat{\boldsymbol{x}}$, can be expressed in terms of these boson averages as

$$M = S - \frac{1}{N}\sum_{\boldsymbol{k}}\langle a^\dagger_{\boldsymbol{k}} a_{\boldsymbol{k}}\rangle \equiv S\left(1 - \frac{T}{SN}\sum_{\boldsymbol{k}}\frac{A_{\boldsymbol{k}}}{\omega^2_{\boldsymbol{k}}}\right). \tag{S9}$$

## B. Interacting spin-waves

To consider the effects of the quartic parts of $\mathcal{H}$ in Eq. S4, $\mathcal{H}_{4,2-2}$, $\mathcal{H}_{4,3-1}$ and $\mathcal{H}_{4,1-3}$, we adopt a mean-field like approach, replacing each possible contraction of operators with averages with respect to the quadratic, or "free" part, $\mathcal{H}_2$ [10, 11]. This procedure produces the same results as leading order perturbation theory in the quartic interactions [12, 13]. For example, consider the scattering term

$$\begin{aligned} a^\dagger_{\boldsymbol{k}+\boldsymbol{q}} a^\dagger_{\boldsymbol{k}'-\boldsymbol{q}} a_{\boldsymbol{k}'} a_{\boldsymbol{k}} \approx\ & \langle a^\dagger_{\boldsymbol{k}+\boldsymbol{q}} a_{\boldsymbol{k}'}\rangle a^\dagger_{\boldsymbol{k}'-\boldsymbol{q}} a_{\boldsymbol{k}} + \langle a^\dagger_{\boldsymbol{k}'-\boldsymbol{q}} a_{\boldsymbol{k}}\rangle a^\dagger_{\boldsymbol{k}+\boldsymbol{q}} a_{\boldsymbol{k}'} \\ & + \langle a^\dagger_{\boldsymbol{k}+\boldsymbol{q}} a_{\boldsymbol{k}}\rangle a^\dagger_{\boldsymbol{k}'-\boldsymbol{q}} a_{\boldsymbol{k}'} + \langle a^\dagger_{\boldsymbol{k}'-\boldsymbol{q}} a_{\boldsymbol{k}'}\rangle a^\dagger_{\boldsymbol{k}+\boldsymbol{q}} a_{\boldsymbol{k}} \\ & + \langle a^\dagger_{\boldsymbol{k}+\boldsymbol{q}} a^\dagger_{\boldsymbol{k}'-\boldsymbol{q}}\rangle a_{\boldsymbol{k}'} a_{\boldsymbol{k}} + \langle a_{\boldsymbol{k}'} a_{\boldsymbol{k}}\rangle a^\dagger_{\boldsymbol{k}+\boldsymbol{q}} a^\dagger_{\boldsymbol{k}'-\boldsymbol{q}}. \end{aligned}$$

Using the fact that the expectation values satisfy $\langle a^\dagger_{\boldsymbol{k}} a_{\boldsymbol{k}'}\rangle \propto \delta_{\boldsymbol{k},\boldsymbol{k}'}$ and $\langle a_{\boldsymbol{k}} a_{\boldsymbol{k}'}\rangle \propto \delta_{\boldsymbol{k},-\boldsymbol{k}'}$, one finds

$$\begin{aligned} a^\dagger_{\boldsymbol{k}+\boldsymbol{q}} a^\dagger_{\boldsymbol{k}'-\boldsymbol{q}} a_{\boldsymbol{k}'} a_{\boldsymbol{k}} \approx\ & \left(\delta_{\boldsymbol{q},\boldsymbol{0}} + \delta_{\boldsymbol{k}+\boldsymbol{q},\boldsymbol{k}'}\right)\left(\langle a^\dagger_{\boldsymbol{k}'} a_{\boldsymbol{k}'}\rangle a^\dagger_{\boldsymbol{k}} a_{\boldsymbol{k}} + \langle a^\dagger_{\boldsymbol{k}} a_{\boldsymbol{k}}\rangle a^\dagger_{\boldsymbol{k}'} a_{\boldsymbol{k}'}\right) \\ & + \delta_{\boldsymbol{k},-\boldsymbol{k}'}\left(\langle a^\dagger_{\boldsymbol{k}+\boldsymbol{q}} a^\dagger_{-\boldsymbol{k}-\boldsymbol{q}}\rangle a_{-\boldsymbol{k}} a_{\boldsymbol{k}} + \langle a_{-\boldsymbol{k}} a_{\boldsymbol{k}}\rangle a^\dagger_{\boldsymbol{k}+\boldsymbol{q}} a^\dagger_{-\boldsymbol{k}-\boldsymbol{q}}\right). \end{aligned}$$

Combining this decomposition with the interaction coefficients $V_{\boldsymbol{k},\boldsymbol{k}',\boldsymbol{q}}$, as specified in Eq. (S5b), gives the expression

$$\begin{aligned} \mathcal{H}_{4,2-2} \approx & \sum_{\boldsymbol{k}}\left(\frac{1}{N}\sum_{\boldsymbol{q}} V_{\boldsymbol{k},\boldsymbol{q},\boldsymbol{0}}\langle a^\dagger_{\boldsymbol{q}} a_{\boldsymbol{q}}\rangle\right) a^\dagger_{\boldsymbol{k}} a_{\boldsymbol{k}} \\ & + \frac{1}{2}\sum_{\boldsymbol{k}}\left\{\left(\frac{1}{2N}\sum_{\boldsymbol{q}} V_{\boldsymbol{q},-\boldsymbol{q},\boldsymbol{k}-\boldsymbol{q}}\langle a_{\boldsymbol{q}} a_{-\boldsymbol{q}}\rangle\right) a^\dagger_{\boldsymbol{k}} a^\dagger_{-\boldsymbol{k}} + \text{H.c.}\right\}, \end{aligned}$$

where $V_{\boldsymbol{k},\boldsymbol{k}',\boldsymbol{k}'-\boldsymbol{k}} = V_{\boldsymbol{k},\boldsymbol{k}',\boldsymbol{0}}$ and $V_{\boldsymbol{k},\boldsymbol{k}',\boldsymbol{0}} = V_{\boldsymbol{k}',\boldsymbol{k},\boldsymbol{0}}$ has been used to simplify the normal term, and shifting the momentum has been used to simplify the anomalous terms. The quartic terms thus appear as corrections to the $A_{\boldsymbol{k}}$ and $B_{\boldsymbol{k}}$ quadratic terms.

Next, consider the same manipulations for the anomalous boson terms, starting with

$$\begin{aligned} a^\dagger_{\boldsymbol{k}} a^\dagger_{\boldsymbol{k}'} a^\dagger_{\boldsymbol{q}} a_{\boldsymbol{k}+\boldsymbol{k}'+\boldsymbol{q}} \approx\ & \langle a^\dagger_{\boldsymbol{k}} a^\dagger_{\boldsymbol{k}'}\rangle a^\dagger_{\boldsymbol{q}} a_{\boldsymbol{k}+\boldsymbol{k}'+\boldsymbol{q}} + a^\dagger_{\boldsymbol{k}} a^\dagger_{\boldsymbol{k}'}\langle a^\dagger_{\boldsymbol{q}} a_{\boldsymbol{k}+\boldsymbol{k}'+\boldsymbol{q}}\rangle \\ & + \langle a^\dagger_{\boldsymbol{k}} a^\dagger_{\boldsymbol{q}}\rangle a^\dagger_{\boldsymbol{k}'} a_{\boldsymbol{k}+\boldsymbol{k}'+\boldsymbol{q}} + a^\dagger_{\boldsymbol{k}} a^\dagger_{\boldsymbol{q}}\langle a^\dagger_{\boldsymbol{k}'} a_{\boldsymbol{k}+\boldsymbol{k}'+\boldsymbol{q}}\rangle \\ & + \langle a^\dagger_{\boldsymbol{k}} a_{\boldsymbol{k}+\boldsymbol{k}'+\boldsymbol{q}}\rangle a^\dagger_{\boldsymbol{k}'} a^\dagger_{\boldsymbol{q}} + a^\dagger_{\boldsymbol{k}} a_{\boldsymbol{k}+\boldsymbol{k}'+\boldsymbol{q}}\langle a^\dagger_{\boldsymbol{k}'} a^\dagger_{\boldsymbol{q}}\rangle. \end{aligned}$$

Using the fact that the expectations in this last equation are diagonal in $\boldsymbol{k}$ (or skew-diagonal) [as in Eq. (S8)], we find

$$\begin{aligned} a^\dagger_{\boldsymbol{k}} a^\dagger_{\boldsymbol{k}'} a^\dagger_{\boldsymbol{q}} a_{\boldsymbol{k}+\boldsymbol{k}'+\boldsymbol{q}} \approx\ & \delta_{\boldsymbol{k},-\boldsymbol{k}'}\left(\langle a^\dagger_{\boldsymbol{k}} a^\dagger_{-\boldsymbol{k}}\rangle a^\dagger_{\boldsymbol{q}} a_{\boldsymbol{q}} + a^\dagger_{\boldsymbol{k}} a^\dagger_{-\boldsymbol{k}}\langle a^\dagger_{\boldsymbol{q}} a_{\boldsymbol{q}}\rangle\right) \\ & + \delta_{\boldsymbol{k},-\boldsymbol{q}}\left(\langle a^\dagger_{\boldsymbol{k}} a^\dagger_{-\boldsymbol{k}}\rangle a^\dagger_{\boldsymbol{k}'} a_{\boldsymbol{k}'} + a^\dagger_{\boldsymbol{k}} a^\dagger_{-\boldsymbol{k}}\langle a^\dagger_{\boldsymbol{k}'} a_{\boldsymbol{k}'}\rangle\right) \\ & + \delta_{\boldsymbol{k}',-\boldsymbol{q}}\left(\langle a^\dagger_{\boldsymbol{k}} a_{\boldsymbol{k}}\rangle a^\dagger_{\boldsymbol{k}'} a^\dagger_{-\boldsymbol{k}'} + a^\dagger_{\boldsymbol{k}} a_{\boldsymbol{k}}\langle a^\dagger_{\boldsymbol{k}'} a^\dagger_{-\boldsymbol{k}'}\rangle\right). \end{aligned}$$

Combining this decomposition with the anomalous interaction coefficients, $D_{\boldsymbol{k},\boldsymbol{k}',\boldsymbol{q}}$ from Eq. (S5c), and using the permutation symmetry of its indices, we find

$$\begin{aligned} \mathcal{H}_{4,3-1} \approx & \sum_{\boldsymbol{k}}\left(\frac{1}{2N}\sum_{\boldsymbol{q}} D_{\boldsymbol{q},-\boldsymbol{q},\boldsymbol{k}}\langle a^\dagger_{\boldsymbol{q}} a^\dagger_{-\boldsymbol{q}}\rangle\right) a^\dagger_{\boldsymbol{k}} a_{\boldsymbol{k}} \\ & + \frac{1}{2}\sum_{\boldsymbol{k}}\left(\frac{1}{N}\sum_{\boldsymbol{q}} D_{\boldsymbol{k},-\boldsymbol{k},\boldsymbol{q}}\langle a^\dagger_{\boldsymbol{q}} a_{\boldsymbol{q}}\rangle\right) a^\dagger_{\boldsymbol{k}} a^\dagger_{-\boldsymbol{k}}. \end{aligned}$$

These terms thus also appear as corrections to $A_{\boldsymbol{k}}$ and $B_{\boldsymbol{k}}$ in the quadratic part of the Hamiltonian. Note that the Hermitian conjugate term of this $\mathcal{H}_{4,3-1}$ also contributes, with its contribution read off from the expression above.

$$\mathcal{H}_{4,1-3} \approx \sum_{\boldsymbol{k}} \left( \frac{1}{2N} \sum_{\boldsymbol{q}} D^*_{\boldsymbol{q},-\boldsymbol{q},\boldsymbol{k}} \langle a_{\boldsymbol{q}} a_{-\boldsymbol{q}} \rangle \right) a^\dagger_{\boldsymbol{k}} a_{\boldsymbol{k}} + \frac{1}{2} \sum_{\boldsymbol{k}} \left( \frac{1}{N} \sum_{\boldsymbol{q}} D^*_{\boldsymbol{k},-\boldsymbol{k},\boldsymbol{q}} \langle a^\dagger_{\boldsymbol{q}} a_{\boldsymbol{q}} \rangle \right) a_{-\boldsymbol{k}} a_{\boldsymbol{k}}.$$

Finally, we can summarize all of these contributions as corrections $\delta A_{\boldsymbol{k}}$ and $\delta B_{\boldsymbol{k}}$ to the original $A_{\boldsymbol{k}}$ and $B_{\boldsymbol{k}}$ of quadratic $\mathcal{H}_2$ origin and write

$$\delta A_{\boldsymbol{k}} = \frac{1}{N} \sum_{\boldsymbol{q}} \left[ V_{\boldsymbol{k},\boldsymbol{q},\boldsymbol{0}} \langle a^\dagger_{\boldsymbol{q}} a_{\boldsymbol{q}} \rangle + \frac{1}{2} \left( D_{\boldsymbol{q},-\boldsymbol{q},\boldsymbol{k}} \langle a^\dagger_{\boldsymbol{q}} a^\dagger_{-\boldsymbol{q}} \rangle + \text{c.c.} \right) \right], \tag{S10a}$$

$$\delta B_{\boldsymbol{k}} = \frac{1}{N} \sum_{\boldsymbol{q}} \left[ D_{\boldsymbol{k},-\boldsymbol{k},\boldsymbol{q}} \langle a^\dagger_{\boldsymbol{q}} a_{\boldsymbol{q}} \rangle + \frac{1}{2} V_{\boldsymbol{q},-\boldsymbol{q},\boldsymbol{k}-\boldsymbol{q}} \langle a_{\boldsymbol{q}} a_{-\boldsymbol{q}} \rangle \right]. \tag{S10b}$$

In terms of these corrections, the renormalized spectrum is given by

$$\Omega_{\boldsymbol{k}} \equiv \sqrt{(A_{\boldsymbol{k}} + \delta A_{\boldsymbol{k}})^2 - (B_{\boldsymbol{k}} + \delta B_{\boldsymbol{k}})^2}. \tag{S11}$$

These corrections can be evaluated using the bare, free (non-interacting) averages from Eq. (S8), though this approach leads to divergences (see Sec. III F). Alternatively, they can be evaluated self-consistently, with the averages in Eq. (S8) computed using $(A_{\boldsymbol{k}} + \delta A_{\boldsymbol{k}})$, $(B_{\boldsymbol{k}} + \delta B_{\boldsymbol{k}})$ and $\Omega_{\boldsymbol{k}}$ instead of $A_{\boldsymbol{k}}$, $B_{\boldsymbol{k}}$ and $\omega_{\boldsymbol{k}}$, a procedure that cures the divergences.

### C. Pseudo-Goldstone gap

The effects of the interactions on the pseudo-Goldstone mode can now be examined. The energy of the $\boldsymbol{k} = \boldsymbol{0}$ mode is given by

$$\Delta \equiv \Omega_{\boldsymbol{0}} = \sqrt{2KS\,(\delta A_{\boldsymbol{0}} + \delta B_{\boldsymbol{0}}) + \delta A_{\boldsymbol{0}}^2 - \delta B_{\boldsymbol{0}}^2}. \tag{S12}$$

For small corrections $\delta A_{\boldsymbol{0}}, \delta B_{\boldsymbol{0}}$, $\Delta$ can be approximated by (the leading term)

$$\Delta \approx \sqrt{2KS}\,\sqrt{\delta A_{\boldsymbol{0}} + \delta B_{\boldsymbol{0}}}. \tag{S13}$$

In the quantum limit where $T \ll \omega_{\boldsymbol{k}}$, the corrections $\delta A_{\boldsymbol{k}}, \delta B_{\boldsymbol{k}}$ are $O(S^0)$ and thus the gap scales as $\Delta \propto \sqrt{S}$. In the classical limit where $T \gg \omega_{\boldsymbol{k}}$, the corrections scale as $\delta A_{\boldsymbol{k}}, \delta B_{\boldsymbol{k}} \sim O(T/S)$ and thus the gap scales as $\Delta \propto \sqrt{T}$, independent of $S$.

### D. Pseudo-Goldstone linewidth

To estimate the scaling of the pseudo-Goldstone mode linewidth with temperature, we consider the magnon self-energy [11] at $\boldsymbol{k} = \boldsymbol{0}$ near $\omega = 0$, $\boldsymbol{\Sigma}(\boldsymbol{0}, 0)$, which takes the form

$$\boldsymbol{\Sigma}(\boldsymbol{0}, 0) \equiv \begin{pmatrix} \delta A_{\boldsymbol{0}} & \delta B_{\boldsymbol{0}} \\ \delta B^*_{\boldsymbol{0}} & \delta A^*_{\boldsymbol{0}} \end{pmatrix},$$

where $\delta A_{\boldsymbol{0}}$ and $\delta B_{\boldsymbol{0}}$ are corrections due to magnon-magnon interactions. Perturbatively, we expect that

$$\delta A_{\boldsymbol{0}} = a_1 T + a_2 T^2 + \cdots, \tag{S14a}$$

$$\delta B_{\boldsymbol{0}} = b_1 T + b_2 T^2 + \cdots, \tag{S14b}$$

where the $O(T)$ corrections (computed in this work) encoded in $a_1$, $b_1$ are both real. The quasi-normal modes, corresponding to the locations of poles of the magnon Green's function [11, 14], are determined from the eigenvalues of $\boldsymbol{\sigma}_z \boldsymbol{M}^{\text{eff}}_{\boldsymbol{0}}$ where

$$\boldsymbol{M}^{\text{eff}}_{\boldsymbol{0}} = \begin{pmatrix} A_{\boldsymbol{0}} + \delta A_{\boldsymbol{0}} & -A_{\boldsymbol{0}} + \delta B_{\boldsymbol{0}} \\ -A_{\boldsymbol{0}} + \delta B^*_{\boldsymbol{0}} & A_{\boldsymbol{0}} + \delta A^*_{\boldsymbol{0}} \end{pmatrix}. \tag{S15}$$

Up to and including terms of $O(T^2)$, the quasi-normal mode frequency is thus given by

$$\operatorname{Re}\Omega_{\boldsymbol{0}} \approx \sqrt{2A_{\boldsymbol{0}}(a_1 + b_1)}\,\sqrt{T} + \left( \frac{a_1^2 - b_1^2 + 2A_{\boldsymbol{0}}(\operatorname{Re} a_2 + \operatorname{Re} b_2)}{4A_{\boldsymbol{0}}(a_1 + b_1)} \right) T^{3/2} + \cdots,$$

$$\operatorname{Im}\Omega_{\boldsymbol{0}} \approx (\operatorname{Im} a_2) T^2 + \cdots.$$

We thus see that the linewidth, determined by $\operatorname{Im}\Omega_{\boldsymbol{0}}$, is expected to scale as $T^2$.

Next, we provide a similar perturbative argument for the scaling relations of the pseudo-Goldstone gap and linewidth with temperature for a type-II pseudo-Goldstone mode as arises, for instance, in the ferromagnetic Heisenberg-compass model on the cubic lattice [9]. For this type-II case, one has $A_{\boldsymbol{0}} = B_{\boldsymbol{0}} = 0$ (in contrast to $|A_{\boldsymbol{0}}| = |B_{\boldsymbol{0}}| \neq 0$ for the type-I case that we focus on in this work), with the magnon-self energy taking the same form as in the type-I case, as discussed in the main text. The poles of the Green's function are determined by the matrix [from Eq. (S15)]

$$\boldsymbol{M}^{\text{eff}}_{\boldsymbol{0}} = \begin{pmatrix} \delta A_{\boldsymbol{0}} & \delta B_{\boldsymbol{0}} \\ \delta B^*_{\boldsymbol{0}} & \delta A^*_{\boldsymbol{0}} \end{pmatrix},$$

with $\delta A_{\boldsymbol{0}}$ and $\delta B_{\boldsymbol{0}}$ taking a similar form as in Eq. (S14). As three-boson terms are absent from the interacting spin-wave Hamiltonian [9], $a_1$ and $b_1$ are real, as in the type-I case. However, generally $a_2$ and $b_2$ can have imaginary parts, producing a spectrum

$$\operatorname{Re}\Omega_{\boldsymbol{0}} \approx \left( \sqrt{a_1^2 - b_1^2} \right) T + \left( \frac{a_1 \operatorname{Re} a_2 - b_1 \operatorname{Re} b_2}{\sqrt{a_1^2 - b_1^2}} \right) T^2 + \cdots,$$

$$\operatorname{Im}\Omega_{\boldsymbol{0}} \approx (\operatorname{Im} a_2) T^2 + \cdots.$$

The leading temperature dependence of the gap is thus predicted to be $\Delta = \operatorname{Re}\Omega_{\boldsymbol{0}} \propto T$, as found from the effective description presented in the main text when applied to a type-II pseudo-Goldstone mode. From $\operatorname{Im}\Omega_{\boldsymbol{0}}$, we obtain a linewidth scaling as $T^2$ for this type-II case, identical to what was found for the type-I pseudo-Goldstone mode.

### E. Self-consistent mean-field theory (SCMFT)

To include the effects of the magnon-magnon interactions self-consistently, we define the "mean-fields"

$$n_{\boldsymbol{k}} \equiv \langle a^\dagger_{\boldsymbol{k}} a_{\boldsymbol{k}} \rangle, \qquad d_{\boldsymbol{k}} \equiv \langle a^\dagger_{\boldsymbol{k}} a^\dagger_{-\boldsymbol{k}} \rangle. \tag{S16}$$

Using Eq. (S10), new values of $n_{\boldsymbol{k}}$ and $d_{\boldsymbol{k}}$ can then be computed by iteratively updating $A_{\boldsymbol{k}}$ and $B_{\boldsymbol{k}}$ to $A'_{\boldsymbol{k}}$ and $B'_{\boldsymbol{k}}$, respectively, with

$$A'_{\boldsymbol{k}} = A_{\boldsymbol{k}} + \frac{1}{N}\sum_{\boldsymbol{q}}\left[V_{\boldsymbol{k},\boldsymbol{q},\boldsymbol{0}} n_{\boldsymbol{q}} + \frac{1}{2}\left(D_{\boldsymbol{q},-\boldsymbol{q},\boldsymbol{k}} d_{\boldsymbol{q}} + D^*_{\boldsymbol{q},-\boldsymbol{q},\boldsymbol{k}} d^*_{\boldsymbol{q}}\right)\right],$$

$$B'_{\boldsymbol{k}} = B_{\boldsymbol{k}} + \frac{1}{N}\sum_{\boldsymbol{q}}\left[D_{\boldsymbol{k},-\boldsymbol{k},\boldsymbol{q}} n_{\boldsymbol{q}} + \frac{1}{2} V_{\boldsymbol{q},-\boldsymbol{q},\boldsymbol{k}-\boldsymbol{q}} d^*_{\boldsymbol{q}}\right],$$

which, using Eq. (S8), results in updated values of $n_{\boldsymbol{k}}$ and $d_{\boldsymbol{k}}$. This process is repeated until the variables $n_{\boldsymbol{k}}$ and $d_{\boldsymbol{k}}$ have converged to the desired precision across the full Brillouin zone.

For the calculations reported here, and in the main text, convergence was considered reached when the sum of all absolute values of the changes in $n_{\boldsymbol{k}}$ and $d_{\boldsymbol{k}}$ in Eq. (S16) over the Brillouin zone between subsequent iterations was less than $10^{-10}$. To launch the iterative process, the mean-fields, $n_{\boldsymbol{k}}$ and $d_{\boldsymbol{k}}$ for each $\boldsymbol{k}$, are initially set to a value of $1/2$, though the precise choice of initial value was found to not affect the final results. Following this approach, we calculate the PG gap for several system sizes, using a discrete sum over the Brillouin zone with $N = L^2$ points. We then extrapolate the gap in the system size to obtain the result in the thermodynamic limit ($N \to \infty$). The finite size scaling of the PG gap using SCMFT is shown in Fig. S2.

### F. Cancellation of divergences in the pseudo-Goldstone gap

Since the non-interacting LSWT spectrum is gapless, we must be mindful of infrared divergent contributions to $\delta A_{\boldsymbol{0}}$ and $\delta B_{\boldsymbol{0}}$. Let us first address this issue in the simplest context, bare perturbation theory in the quartic interactions.

We focus on the classical limit where $\omega_{\boldsymbol{k}} \ll T$, but similar considerations apply in the full quantum case at finite temperature; since $\omega_{\boldsymbol{k}} \to 0$ as $\boldsymbol{k} \to \boldsymbol{0}$, there is always a regime in $\boldsymbol{k}$ near the zone center where the frequency is small relative to temperature, even in the quantum limit. Consider the corrections, Eq. (S10), in the thermodynamic limit ($N \to \infty$), replacing the discrete sums with integrals. At $\boldsymbol{k} = \boldsymbol{0}$, this gives [using Eq. (S8)]

$$\delta A_{\boldsymbol{0}} = \int \frac{d^2q}{(2\pi)^2}\frac{T}{\omega^2_{\boldsymbol{q}}}\left[V_{\boldsymbol{0},\boldsymbol{q},\boldsymbol{0}} A_{\boldsymbol{q}} - D_{\boldsymbol{q},-\boldsymbol{q},\boldsymbol{0}} B_{\boldsymbol{q}}\right], \tag{S17a}$$

$$\delta B_{\boldsymbol{0}} = \int \frac{d^2q}{(2\pi)^2}\frac{T}{\omega^2_{\boldsymbol{q}}}\left[D_{\boldsymbol{0},\boldsymbol{0},\boldsymbol{q}} A_{\boldsymbol{q}} - \frac{1}{2} V_{\boldsymbol{q},-\boldsymbol{q},-\boldsymbol{q}} B_{\boldsymbol{q}}\right], \tag{S17b}$$

where the integral is over the Brillouin zone $-\pi \le q_x, q_y \le \pi$ (the lattice spacing has been set to one). At small $\boldsymbol{q}$, the spectrum is approximately linear in $\boldsymbol{q}$ with

$$\omega_{\boldsymbol{q}} = S\sqrt{2K\left(J|\boldsymbol{q}|^2 + Kq_y^2\right)} + O(|\boldsymbol{q}|^2)$$

and thus the factor $T/\omega^2_{\boldsymbol{q}} \propto 1/|\boldsymbol{q}|^2$ is singular as $|\boldsymbol{q}| \to 0$. The numerators (the coefficients of the $T/\omega^2_{\boldsymbol{q}}$ terms) in Eq. (S17) remain finite in this limit, with

$$V_{\boldsymbol{0},\boldsymbol{q},\boldsymbol{0}} A_{\boldsymbol{q}} - D_{\boldsymbol{q},-\boldsymbol{q},\boldsymbol{0}} B_{\boldsymbol{q}} = -\frac{SK^2}{2} + O(|\boldsymbol{q}|^2),$$

$$D_{\boldsymbol{0},\boldsymbol{0},\boldsymbol{q}} A_{\boldsymbol{q}} - \frac{1}{2} V_{\boldsymbol{q},-\boldsymbol{q},-\boldsymbol{q}} B_{\boldsymbol{q}} = +\frac{SK^2}{2} + O(|\boldsymbol{q}|^2).$$

One therefore finds that both $\delta A_{\boldsymbol{0}}$ and $\delta B_{\boldsymbol{0}}$ are logarithmically divergent. Explicitly, integrating over a region $2\pi/L < |\boldsymbol{q}| < \Lambda \ll \pi$

$$\int_{2\pi/L<|\boldsymbol{q}|<\Lambda} \frac{d^2q}{(2\pi)^2}\frac{1}{\omega^2_{\boldsymbol{q}}} = \frac{1}{4\pi S^2 K\sqrt{J(J+K)}}\ln\left(\frac{L\Lambda}{2\pi}\right). \tag{S18}$$

Since the upper cutoff is chosen to satisfy $\Lambda \ll \pi$, the divergent contributions to $\delta A_{\boldsymbol{0}}$ and $\delta B_{\boldsymbol{0}}$ take the form

$$\delta A_{\boldsymbol{0}} = -\frac{TK\ln L}{8\pi S\sqrt{J(J+K)}} + (\text{reg.}), \tag{S19a}$$

$$\delta B_{\boldsymbol{0}} = +\frac{TK\ln L}{8\pi S\sqrt{J(J+K)}} + (\text{reg.}), \tag{S19b}$$

where (reg.) stands for terms that remain finite as $L \to \infty$. Interestingly, while $\delta A_0$ and $\delta B_0$ are each $\ln L$ divergent, the *sum* ($\delta A_{\boldsymbol{0}} + \delta B_{\boldsymbol{0}}$) which appears in the expression for the pseudo-Goldstone gap [Eq. (S13)], $\Delta$, is finite. This can be made more explicit by carrying out the same expansions for ($\delta A_{\boldsymbol{0}} + \delta B_{\boldsymbol{0}}$),

$$\delta A_{\boldsymbol{0}} + \delta B_{\boldsymbol{0}} = \int \frac{d^2q}{(2\pi)^2}\frac{T}{\omega^2_{\boldsymbol{q}}}\left[2K^2S(q_x^2 - q_y^2) + O(|\boldsymbol{q}|^4)\right]. \tag{S20}$$

The $O(|\boldsymbol{q}|^2)$ term in the $\omega^2_{\boldsymbol{q}}$ denominator is thus compensated by a corresponding $O(|\boldsymbol{q}|^2)$ term in the numerator of Eq. (S20). However, note that this cancellation *only occurs at leading order* in $\delta A_{\boldsymbol{0}}$, $\delta B_{\boldsymbol{0}}$. The complete expression $\sqrt{(A_{\boldsymbol{0}} + \delta A_{\boldsymbol{0}})^2 - (B_{\boldsymbol{0}} + \delta B_{\boldsymbol{0}})^2}$, which incorporates higher-order contributions, remains logarithmically divergent. Similarly, the leading corrections from bare perturbation theory to $\Omega_{\boldsymbol{k}}$ at *non-zero* $\boldsymbol{k}$ are also divergent.

Since the bare perturbation theory diverges, except for the leading temperature dependence of the PG gap at $\boldsymbol{q} = \boldsymbol{0}$, in order to obtain the full temperature dependence of the interaction corrections to $\Omega_{\boldsymbol{q}}$, we proceed with a self-consistent approach. This way, the equation for the corrections $\delta A_{\boldsymbol{0}}$ and $\delta B_{\boldsymbol{0}}$ become

$$\delta A_{\boldsymbol{0}} = \int \frac{d^2q}{(2\pi)^2}\frac{T}{\Omega^2_{\boldsymbol{q}}}\left[V_{\boldsymbol{0},\boldsymbol{q},\boldsymbol{0}}(A_{\boldsymbol{q}} + \delta A_{\boldsymbol{q}}) - D_{\boldsymbol{q},-\boldsymbol{q},\boldsymbol{0}}(B_{\boldsymbol{q}} + \delta B_{\boldsymbol{q}})\right],$$

$$\delta B_{\boldsymbol{0}} = \int \frac{d^2q}{(2\pi)^2}\frac{T}{\Omega^2_{\boldsymbol{q}}}\left[D_{\boldsymbol{0},\boldsymbol{0},\boldsymbol{q}}(A_{\boldsymbol{q}} + \delta A_{\boldsymbol{q}}) - \frac{1}{2} V_{\boldsymbol{q},-\boldsymbol{q},-\boldsymbol{q}}(B_{\boldsymbol{q}} + \delta B_{\boldsymbol{q}})\right],$$

where the renormalized spectrum $\Omega_{\boldsymbol{q}}$ arises from evaluating the averages in Eq. (S8) self-consistently. In such a self-consistent mean-field theory, the spectrum $\Omega_{\boldsymbol{q}}$ "already" contains a finite gap at $\boldsymbol{q} = \boldsymbol{0}$. The gap acts as an effective infrared

cutoff rendering the integrals in Eq. (S18) finite. The disappearance of the divergence then manifests itself in the cancellation of the leading (self-consistent) dependence on the gap $\Delta$.

To see this explicitly, consider the self-consistent spectrum which, for small $\boldsymbol{q}$, takes the form

$$\Omega_{\boldsymbol{q}} = \sqrt{2KS^2\left(J|\boldsymbol{q}|^2 + Kq_y^2\right) + \Delta^2} + O(|\boldsymbol{q}|^2).$$

For sufficiently small $\Delta$, the integration region can be divided into two parts: $|\boldsymbol{q}| \gtrsim k_0$ and $|\boldsymbol{q}| \lesssim k_0$ such that

$$\Omega_{\boldsymbol{q}} \approx \begin{cases} \Delta, & |\boldsymbol{q}| \lesssim k_0, \\ S\sqrt{2K\left(J|\boldsymbol{q}|^2 + Kq_y^2\right)}, & |\boldsymbol{q}| \gtrsim k_0. \end{cases}$$

Roughly, the boundary separating these regions scales as

$$k_0 \sim \frac{\Delta}{SK} \propto \sqrt{T} \tag{S22}$$

when $K \gtrsim J$. Alternatively, $k_0$ is the wave-vector at which the bare spectrum $\omega_{\boldsymbol{k}}$ becomes comparable to the interaction induced gap, $\Delta$. The primary change to the spectrum, and thus to $\delta A_{\boldsymbol{0}}$ and $\delta B_{\boldsymbol{0}}$, occurs for $|\boldsymbol{q}| < k_0$. Carrying out the integration in Eq. (S18) over the region responsible for its divergent contributions, we find they are rendered finite. Explicitly,

$$\int_{k_0<|\boldsymbol{q}|<\Lambda} \frac{d^2q}{(2\pi)^2}\frac{1}{\Omega_{\boldsymbol{q}}^2} \sim \frac{\ln(KS\Lambda/\Delta)}{4\pi S^2 K\sqrt{J(J+K)}}.$$

Given that $\Delta \propto \sqrt{T}$, this contribution to the integral now scales as $-\ln T$. Thus the divergence has been cured in the individual corrections $\delta A_{\boldsymbol{0}}$ and $\delta B_{\boldsymbol{0}}$. We note that the $\ln(\Lambda/\Delta) \sim -\ln T$ terms cancel in the sum $(\delta A_{\boldsymbol{0}} + \delta B_{\boldsymbol{0}})$ which controls the leading contribution to the gap [similarly to Eq. (S13)] and the result from bare perturbation theory is recovered. In this way, bare perturbation theory for the asymptotic $\sqrt{T}$ scaling of the pseudo-Goldstone gap is well-defined and divergence free, and matches the results from the SCMFT calculations. Note that the region $0 < |\boldsymbol{q}| < k_0$ gives only a finite contribution that goes as

$$\int_{0<|\boldsymbol{q}|<k_0} \frac{d^2q}{(2\pi)^2}\frac{1}{\Omega_{\boldsymbol{q}}^2} \sim \frac{k_0^2}{4\pi\Delta^2} \sim \text{const.}\,,$$

since $k_0 \propto \Delta$ from Eq. (S22).

### G. Logarithmic corrections to magnetization

While the contributions $\propto \ln T$ cancel in the leading order correction in $\delta A_{\boldsymbol{0}}$, $\delta B_{\boldsymbol{0}}$ to $\Delta$, they reappear explicitly in static quantities such as the magnetization. In the classical limit, the net magnetization [Eq. (S9)] is given by

$$M = S - T\int \frac{d^2k}{(2\pi)^2}\frac{A_{\boldsymbol{k}}}{\omega_{\boldsymbol{k}}^2}, \tag{S23}$$

in the thermodynamic limit ($N \to \infty$). Like the bare corrections $\delta A_{\boldsymbol{0}}$ and $\delta B_{\boldsymbol{0}}$ in Eq. (S17), in LSWT, $M$ has a logarithmic infrared divergence, given that $\omega_{\boldsymbol{k}}$ scales linearly with $\boldsymbol{k}$ at small $|\boldsymbol{k}|$, while $A_{\boldsymbol{k}}$ tends to the constant $A_{\boldsymbol{0}} = KS$. Naïvely, this would indicate the destruction of the long-range ferromagnetic order, as happens when there is a true symmetry-protected Goldstone mode [15].

To resolve this divergence, we must include the dynamically generated pseudo-Goldstone gap. The expression for $M$ in the SCMFT can be obtained from Eq. (S23), via the replacements $\omega_{\boldsymbol{k}} \to \Omega_{\boldsymbol{k}}$ and $A_{\boldsymbol{k}} \to A_{\boldsymbol{k}} + \delta A_{\boldsymbol{k}}$. Explicitly,

$$M = S - T\int \frac{d^2k}{(2\pi)^2}\frac{A_{\boldsymbol{k}} + \delta A_{\boldsymbol{k}}}{\Omega_{\boldsymbol{k}}^2}, \tag{S24}$$

where, again, $\Omega_{\boldsymbol{k}}$ is the self-consistent spectrum with pseudo-Goldstone gap $\Delta$. Following the same strategy as in Sec. III F, we approximate the self-consistent spectrum, $\Omega_{\boldsymbol{k}}$, over the three pertinent regions of reciprocal space

$$\Omega_{\boldsymbol{k}} \approx \begin{cases} \Delta, & 0 < |\boldsymbol{k}| \lesssim k_0, \\ S\sqrt{2K\left(J|\boldsymbol{k}|^2 + Kk_y^2\right)}, & k_0 \lesssim |\boldsymbol{k}| \lesssim \Lambda, \\ \omega_{\boldsymbol{k}}. & |\boldsymbol{k}| \gtrsim \Lambda. \end{cases} \tag{S25}$$

The integral defining $M$ is then split into three parts

$$\int \frac{d^2k}{(2\pi)^2} = \int_{0<|\boldsymbol{k}|<k_0} \frac{d^2k}{(2\pi)^2} + \int_{k_0<|\boldsymbol{k}|<\Lambda} \frac{d^2k}{(2\pi)^2} + \int_{|\boldsymbol{k}|>\Lambda} \frac{d^2k}{(2\pi)^2}.$$

The first and second integrals depend on temperature through $\Delta \propto \sqrt{T}$ and $k_0 \sim \Delta/(KS)$ [see Eq. (S22)]. The last integral is over wave-vectors large enough such that the interaction corrections are minor and, therefore, this contribution to the integral has no additional temperature dependence. The correction to $M$ in Eq. (S24) arising from this last (third) term is thus $\propto T$ (from the integral prefactor).

For the region $|\boldsymbol{k}| \lesssim \Lambda$, we approximate $A_{\boldsymbol{k}} + \delta A_{\boldsymbol{k}} \approx KS$, leaving the two contributions

$$\int_{0<|\boldsymbol{k}|<k_0} \frac{d^2k}{(2\pi)^2}\frac{KST}{\Delta^2} = \frac{T}{4\pi KS},$$

$$\int_{k_0<|\boldsymbol{k}|<\Lambda} \frac{d^2k}{(2\pi)^2}\frac{KST}{2KS^2\left(J|\boldsymbol{k}|^2 + Kk_y^2\right)} = \frac{T\ln(KS\Lambda/\Delta)}{4\pi S\sqrt{J(J+K)}}.$$

The renormalized spectrum thus yields two additional contributions to $M$: one that adds an additional part $\propto T$ and another new, and perhaps most interesting, part, $\propto T\ln T$, and where we used $\Delta \propto \sqrt{T}$.

To summarize, the magnetization at low temperatures takes the form

$$M = S - c_1 T - c_2 T\ln T + \cdots, \tag{S26}$$

where $c_1$ and $c_2$ are temperature independent constants. The logarithmic $T\ln T$ dependence arises from the temperature dependence of the pseudo-Goldstone gap, $\Delta$. As $T \to 0$, both of these temperature dependent terms go to zero (as it should classically) and the system becomes fully polarized with $M \to S$. Hence true long-range order is induced by ObTD, with the lurking infrared divergences tamed by the ObTD-induced PG gap, $\Delta$.

[1] J. D. Alzate-Cardona, D. Sabogal-Suárez, R. F. L. Evans, and E. Restrepo-Parra, "Optimal phase space sampling for Monte Carlo simulations of Heisenberg spin systems," Journal of Physics: Condensed Matter **31**, 095802 (2019).

[2] Michael Creutz, "Overrelaxation and Monte Carlo simulation," Phys. Rev. D **36**, 515–519 (1987).

[3] M. E. J. Newman and G. T. Barkema, *Monte Carlo methods in statistical physics* (Clarendon Press, Oxford, 1999).

[4] J. R. Dormand and P. J. Prince, "A family of embedded Runge-Kutta formulae," Journal of Computational and Applied Mathematics **6**, 19–26 (1980).

[5] K. Ahnert and M. Mulansky, "Odeint – solving ordinary differential equations in C++," AIP Conference Proceedings **1389**, 1586–1589 (2011).

[6] K. Ahnert and M. Mulansky, "Boost C++ Library: Odeint," (2012).

[7] J. C. Bowman and M. Roberts, "FFTW++: A fast Fourier transform C++ header class for the FFTW3 library," (2010).

[8] A. Auerbach, *Interacting Electrons and Quantum Magnetism*, Graduate Texts in Contemporary Physics (Springer New York, 1998).

[9] Jeffrey G. Rau, Paul A. McClarty, and Roderich Moessner, "Pseudo-Goldstone gaps and order-by-quantum disorder in frustrated magnets," Phys. Rev. Lett. **121**, 237201 (2018).

[10] H. Bruus and K. Flensberg, *Many-Body Quantum Theory in Condensed Matter Physics: An Introduction*, Oxford Graduate Texts (Oxford University Press, Oxford, 2004).

[11] J.P. Blaizot and G. Ripka, *Quantum Theory of Finite Systems* (MIT Press, Cambridge, 1986).

[12] P. D. Loly, "The Heisenberg ferromagnet in the selfconsistently renormalized spin wave approximation," Journal of Physics C: Solid State Physics **4**, 1365–1377 (1971).

[13] A. V. Chubukov, S. Sachdev, and T. Senthil, "Large-$S$ expansion for quantum antiferromagnets on a triangular lattice," Journal of Physics: Condensed Matter **6**, 8891–8902 (1994).

[14] M. E. Zhitomirsky and A. L. Chernyshev, "Colloquium: Spontaneous magnon decays," Rev. Mod. Phys. **85**, 219–242 (2013).

[15] P. M. Chaikin and T. C. Lubensky, *Principles of Condensed Matter Physics* (Cambridge University Press, 1995).
